# Supplementary material for: Deep Neural Network for DrawiNg Networks, (DNN)^2
Source: arXiv:2108.03632 source file (2021-08-10)
Supplement: Supplementary file 1 [file stats.tex]

\subsection{Training methods evaluation}
\label{sec:bench1}
\begin{table}[!h]
\centering
\caption{Performances ($average \pm standard\:deviation$) of the different $(DNN)^2$ instances compared in Section 4.4.}
\resizebox{\columnwidth}{!}{
\begin{tabular}{lllllll}
\toprule
{} &                                 Stress &              \makecell{Aspect\\ ratio} &                 \makecell{Cross.\\ number} &              \makecell{Angular\\ res.} &           \makecell{Cluster\\ overlap} &             \makecell{Neighb.\\ pres.} \\
                                                &                                        &                                        &                                            &                                        &                                        &                                        \\
\midrule
\makecell{finetuned\\ $(DNN)^{2\textbf{*}}$}    &  \makecell{$0.115$ \\ $\pm$ \\$0.046$} &  \makecell{$0.229$ \\ $\pm$ \\$0.105$} &    \makecell{$30.625$ \\ $\pm$ \\$34.824$} &  \makecell{$0.917$ \\ $\pm$ \\$0.138$} &  \makecell{$0.541$ \\ $\pm$ \\$0.206$} &  \makecell{$0.409$ \\ $\pm$ \\$0.136$} \\
\midrule
\makecell{finetuned\\ $(DNN)^{2}$}              &   \makecell{$0.128$ \\ $\pm$ \\$0.06$} &  \makecell{$0.294$ \\ $\pm$ \\$0.134$} &    \makecell{$36.343$ \\ $\pm$ \\$39.879$} &  \makecell{$0.969$ \\ $\pm$ \\$0.092$} &   \makecell{$0.58$ \\ $\pm$ \\$0.197$} &  \makecell{$0.468$ \\ $\pm$ \\$0.154$} \\
\midrule
\makecell{from scratch\\ $(DNN)^{2\textbf{*}}$} &  \makecell{$0.119$ \\ $\pm$ \\$0.058$} &  \makecell{$0.278$ \\ $\pm$ \\$0.149$} &     \makecell{$36.08$ \\ $\pm$ \\$38.282$} &  \makecell{$0.973$ \\ $\pm$ \\$0.084$} &  \makecell{$0.587$ \\ $\pm$ \\$0.189$} &  \makecell{$0.481$ \\ $\pm$ \\$0.153$} \\
\midrule
\makecell{from scratch\\ $(DNN)^{2}$}           &  \makecell{$0.127$ \\ $\pm$ \\$0.061$} &  \makecell{$0.295$ \\ $\pm$ \\$0.134$} &     \makecell{$38.41$ \\ $\pm$ \\$41.346$} &  \makecell{$0.971$ \\ $\pm$ \\$0.084$} &  \makecell{$0.589$ \\ $\pm$ \\$0.192$} &  \makecell{$0.484$ \\ $\pm$ \\$0.157$} \\
\midrule
\makecell{pretrained\\ $(DNN)^{2\textbf{*}}$}   &   \makecell{$0.632$ \\ $\pm$ \\$0.44$} &  \makecell{$0.156$ \\ $\pm$ \\$0.066$} &  \makecell{$203.135$ \\ $\pm$ \\$192.254$} &  \makecell{$0.945$ \\ $\pm$ \\$0.092$} &  \makecell{$0.707$ \\ $\pm$ \\$0.204$} &    \makecell{$0.8$ \\ $\pm$ \\$0.155$} \\
\midrule
\makecell{pretrained\\ $(DNN)^{2}$}             &  \makecell{$0.584$ \\ $\pm$ \\$0.384$} &  \makecell{$0.163$ \\ $\pm$ \\$0.063$} &  \makecell{$180.188$ \\ $\pm$ \\$173.418$} &  \makecell{$0.945$ \\ $\pm$ \\$0.108$} &    \makecell{$0.695$ \\ $\pm$ \\$0.2$} &  \makecell{$0.798$ \\ $\pm$ \\$0.148$} \\
\bottomrule
\end{tabular}
}
\end{table}
\begin{table}[!h]
\centering
\caption{Conover-Iman post-hoc test p-values for Stress in Section 4.4. Significant threshold is $\alpha = 0.05$.}
\resizebox{\columnwidth}{!}{
\begin{tabular}{lllllll}
\toprule
{} & \makecell{finetuned\\ $(DNN)^{2\textbf{*}}$} & \makecell{finetuned\\ $(DNN)^{2}$} & \makecell{from scratch\\ $(DNN)^{2\textbf{*}}$} & \makecell{from scratch\\ $(DNN)^{2}$} & \makecell{pretrained\\ $(DNN)^{2\textbf{*}}$} & \makecell{pretrained\\ $(DNN)^{2}$} \\
\midrule
\makecell{finetuned\\ $(DNN)^{2\textbf{*}}$}    &                                              &                                0.0 &                                           0.093 &                                 0.000 &                                           0.0 &                               0.000 \\
\makecell{finetuned\\ $(DNN)^{2}$}              &                                              &                                    &                                           0.000 &                                 0.399 &                                           0.0 &                               0.000 \\
\makecell{from scratch\\ $(DNN)^{2\textbf{*}}$} &                                              &                                    &                                                 &                                 0.000 &                                           0.0 &                               0.000 \\
\makecell{from scratch\\ $(DNN)^{2}$}           &                                              &                                    &                                                 &                                       &                                           0.0 &                               0.000 \\
\makecell{pretrained\\ $(DNN)^{2\textbf{*}}$}   &                                              &                                    &                                                 &                                       &                                               &                               0.121 \\
\makecell{pretrained\\ $(DNN)^{2}$}             &                                              &                                    &                                                 &                                       &                                               &                                     \\
\bottomrule
\end{tabular}
}
\end{table}
\begin{table}[!h]
\centering
\caption{Conover-Iman post-hoc test p-values for Aspect ratio in Section 4.4. Significant threshold is $\alpha = 0.05$.}
\resizebox{\columnwidth}{!}{
\begin{tabular}{lllllll}
\toprule
{} & \makecell{finetuned\\ $(DNN)^{2\textbf{*}}$} & \makecell{finetuned\\ $(DNN)^{2}$} & \makecell{from scratch\\ $(DNN)^{2\textbf{*}}$} & \makecell{from scratch\\ $(DNN)^{2}$} & \makecell{pretrained\\ $(DNN)^{2\textbf{*}}$} & \makecell{pretrained\\ $(DNN)^{2}$} \\
\midrule
\makecell{finetuned\\ $(DNN)^{2\textbf{*}}$}    &                                              &                                0.0 &                                             0.0 &                                 0.000 &                                           0.0 &                               0.000 \\
\makecell{finetuned\\ $(DNN)^{2}$}              &                                              &                                    &                                             0.0 &                                 0.422 &                                           0.0 &                               0.000 \\
\makecell{from scratch\\ $(DNN)^{2\textbf{*}}$} &                                              &                                    &                                                 &                                 0.000 &                                           0.0 &                               0.000 \\
\makecell{from scratch\\ $(DNN)^{2}$}           &                                              &                                    &                                                 &                                       &                                           0.0 &                               0.000 \\
\makecell{pretrained\\ $(DNN)^{2\textbf{*}}$}   &                                              &                                    &                                                 &                                       &                                               &                               0.001 \\
\makecell{pretrained\\ $(DNN)^{2}$}             &                                              &                                    &                                                 &                                       &                                               &                                     \\
\bottomrule
\end{tabular}
}
\end{table}
\begin{table}[!h]
\centering
\caption{Conover-Iman post-hoc test p-values for Cross. number in Section 4.4. Significant threshold is $\alpha = 0.05$.}
\resizebox{\columnwidth}{!}{
\begin{tabular}{lllllll}
\toprule
{} & \makecell{finetuned\\ $(DNN)^{2\textbf{*}}$} & \makecell{finetuned\\ $(DNN)^{2}$} & \makecell{from scratch\\ $(DNN)^{2\textbf{*}}$} & \makecell{from scratch\\ $(DNN)^{2}$} & \makecell{pretrained\\ $(DNN)^{2\textbf{*}}$} & \makecell{pretrained\\ $(DNN)^{2}$} \\
\midrule
\makecell{finetuned\\ $(DNN)^{2\textbf{*}}$}    &                                              &                                0.0 &                                           0.000 &                                 0.000 &                                           0.0 &                                0.00 \\
\makecell{finetuned\\ $(DNN)^{2}$}              &                                              &                                    &                                           0.718 &                                 0.140 &                                           0.0 &                                0.00 \\
\makecell{from scratch\\ $(DNN)^{2\textbf{*}}$} &                                              &                                    &                                                 &                                 0.264 &                                           0.0 &                                0.00 \\
\makecell{from scratch\\ $(DNN)^{2}$}           &                                              &                                    &                                                 &                                       &                                           0.0 &                                0.00 \\
\makecell{pretrained\\ $(DNN)^{2\textbf{*}}$}   &                                              &                                    &                                                 &                                       &                                               &                                0.02 \\
\makecell{pretrained\\ $(DNN)^{2}$}             &                                              &                                    &                                                 &                                       &                                               &                                     \\
\bottomrule
\end{tabular}
}
\end{table}
\begin{table}[!h]
\centering
\caption{Conover-Iman post-hoc test p-values for Angular res. in Section 4.4. Significant threshold is $\alpha = 0.05$.}
\resizebox{\columnwidth}{!}{
\begin{tabular}{lllllll}
\toprule
{} & \makecell{finetuned\\ $(DNN)^{2\textbf{*}}$} & \makecell{finetuned\\ $(DNN)^{2}$} & \makecell{from scratch\\ $(DNN)^{2\textbf{*}}$} & \makecell{from scratch\\ $(DNN)^{2}$} & \makecell{pretrained\\ $(DNN)^{2\textbf{*}}$} & \makecell{pretrained\\ $(DNN)^{2}$} \\
\midrule
\makecell{finetuned\\ $(DNN)^{2\textbf{*}}$}    &                                              &                                0.0 &                                             0.0 &                                   0.0 &                                           0.0 &                                 0.0 \\
\makecell{finetuned\\ $(DNN)^{2}$}              &                                              &                                    &                                             0.0 &                                   0.0 &                                           0.0 &                                 0.0 \\
\makecell{from scratch\\ $(DNN)^{2\textbf{*}}$} &                                              &                                    &                                                 &                                   0.0 &                                           0.0 &                                 0.0 \\
\makecell{from scratch\\ $(DNN)^{2}$}           &                                              &                                    &                                                 &                                       &                                           0.0 &                                 0.0 \\
\makecell{pretrained\\ $(DNN)^{2\textbf{*}}$}   &                                              &                                    &                                                 &                                       &                                               &                                 0.0 \\
\makecell{pretrained\\ $(DNN)^{2}$}             &                                              &                                    &                                                 &                                       &                                               &                                     \\
\bottomrule
\end{tabular}
}
\end{table}
\begin{table}[!h]
\centering
\caption{Conover-Iman post-hoc test p-values for Cluster overlap in Section 4.4. Significant threshold is $\alpha = 0.05$.}
\resizebox{\columnwidth}{!}{
\begin{tabular}{lllllll}
\toprule
{} & \makecell{finetuned\\ $(DNN)^{2\textbf{*}}$} & \makecell{finetuned\\ $(DNN)^{2}$} & \makecell{from scratch\\ $(DNN)^{2\textbf{*}}$} & \makecell{from scratch\\ $(DNN)^{2}$} & \makecell{pretrained\\ $(DNN)^{2\textbf{*}}$} & \makecell{pretrained\\ $(DNN)^{2}$} \\
\midrule
\makecell{finetuned\\ $(DNN)^{2\textbf{*}}$}    &                                              &                                0.0 &                                           0.000 &                                 0.000 &                                           0.0 &                               0.000 \\
\makecell{finetuned\\ $(DNN)^{2}$}              &                                              &                                    &                                           0.602 &                                 0.129 &                                           0.0 &                               0.000 \\
\makecell{from scratch\\ $(DNN)^{2\textbf{*}}$} &                                              &                                    &                                                 &                                 0.319 &                                           0.0 &                               0.000 \\
\makecell{from scratch\\ $(DNN)^{2}$}           &                                              &                                    &                                                 &                                       &                                           0.0 &                               0.000 \\
\makecell{pretrained\\ $(DNN)^{2\textbf{*}}$}   &                                              &                                    &                                                 &                                       &                                               &                               0.005 \\
\makecell{pretrained\\ $(DNN)^{2}$}             &                                              &                                    &                                                 &                                       &                                               &                                     \\
\bottomrule
\end{tabular}
}
\end{table}
\begin{table}[!h]
\centering
\caption{Conover-Iman post-hoc test p-values for Neighb. pres. in Section 4.4. Significant threshold is $\alpha = 0.05$.}
\resizebox{\columnwidth}{!}{
\begin{tabular}{lllllll}
\toprule
{} & \makecell{finetuned\\ $(DNN)^{2\textbf{*}}$} & \makecell{finetuned\\ $(DNN)^{2}$} & \makecell{from scratch\\ $(DNN)^{2\textbf{*}}$} & \makecell{from scratch\\ $(DNN)^{2}$} & \makecell{pretrained\\ $(DNN)^{2\textbf{*}}$} & \makecell{pretrained\\ $(DNN)^{2}$} \\
\midrule
\makecell{finetuned\\ $(DNN)^{2\textbf{*}}$}    &                                              &                                0.0 &                                           0.000 &                                 0.000 &                                           0.0 &                               0.000 \\
\makecell{finetuned\\ $(DNN)^{2}$}              &                                              &                                    &                                           0.007 &                                 0.000 &                                           0.0 &                               0.000 \\
\makecell{from scratch\\ $(DNN)^{2\textbf{*}}$} &                                              &                                    &                                                 &                                 0.338 &                                           0.0 &                               0.000 \\
\makecell{from scratch\\ $(DNN)^{2}$}           &                                              &                                    &                                                 &                                       &                                           0.0 &                               0.000 \\
\makecell{pretrained\\ $(DNN)^{2\textbf{*}}$}   &                                              &                                    &                                                 &                                       &                                               &                               0.785 \\
\makecell{pretrained\\ $(DNN)^{2}$}             &                                              &                                    &                                                 &                                       &                                               &                                     \\
\bottomrule
\end{tabular}
}
\end{table}
\clearpage\subsection{Comparison with \textit{tsNET}}
\label{sec:bench2}
\begin{table}[!h]
\centering
\caption{Performances ($average \pm standard\:deviation$) of the different $(DNN)^2$ instances compared in Section 4.5.}
\resizebox{\columnwidth}{!}{
\begin{tabular}{llllllll}
\toprule
{} &                                 Stress &              \makecell{Aspect\\ ratio} &               \makecell{Cross.\\ number} &              \makecell{Angular\\ res.} &           \makecell{Cluster\\ overlap} &             \makecell{Neighb.\\ pres.} &                  \makecell{Execution\\ time} \\
                                             &                                        &                                        &                                          &                                        &                                        &                                        &                                              \\
\midrule
$tsNET$                                      &  \makecell{$0.144$ \\ $\pm$ \\$0.155$} &  \makecell{$0.191$ \\ $\pm$ \\$0.091$} &  \makecell{$27.652$ \\ $\pm$ \\$31.753$} &  \makecell{$0.885$ \\ $\pm$ \\$0.155$} &  \makecell{$0.489$ \\ $\pm$ \\$0.229$} &    \makecell{$0.407$ \\ $\pm$ \\$0.1$} &  \makecell{$6541.891$ \\ $\pm$ \\$5068.464$} \\
\midrule
$tsNET^*$                                    &  \makecell{$0.124$ \\ $\pm$ \\$0.049$} &  \makecell{$0.206$ \\ $\pm$ \\$0.109$} &  \makecell{$27.126$ \\ $\pm$ \\$31.972$} &  \makecell{$0.872$ \\ $\pm$ \\$0.181$} &   \makecell{$0.49$ \\ $\pm$ \\$0.218$} &  \makecell{$0.386$ \\ $\pm$ \\$0.115$} &  \makecell{$5836.112$ \\ $\pm$ \\$5933.273$} \\
\midrule
\makecell{finetuned\\ $(DNN)^{2\textbf{*}}$} &  \makecell{$0.111$ \\ $\pm$ \\$0.042$} &  \makecell{$0.229$ \\ $\pm$ \\$0.104$} &   \makecell{$29.971$ \\ $\pm$ \\$35.65$} &   \makecell{$0.905$ \\ $\pm$ \\$0.15$} &  \makecell{$0.507$ \\ $\pm$ \\$0.214$} &   \makecell{$0.397$ \\ $\pm$ \\$0.14$} &        \makecell{$24.808$ \\ $\pm$ \\$8.61$} \\
\midrule
\makecell{finetuned\\ $(DNN)^{2}$}           &  \makecell{$0.117$ \\ $\pm$ \\$0.041$} &    \makecell{$0.3$ \\ $\pm$ \\$0.136$} &   \makecell{$34.865$ \\ $\pm$ \\$40.48$} &  \makecell{$0.963$ \\ $\pm$ \\$0.101$} &   \makecell{$0.55$ \\ $\pm$ \\$0.207$} &  \makecell{$0.451$ \\ $\pm$ \\$0.159$} &      \makecell{$20.427$ \\ $\pm$ \\$10.388$} \\
\bottomrule
\end{tabular}
}
\end{table}
\begin{table}[!h]
\centering
\caption{Conover-Iman post-hoc test p-values for Stress in Section 4.5. Significant threshold is $\alpha = 0.05$.}
\resizebox{\columnwidth}{!}{
\begin{tabular}{lllll}
\toprule
{} & $tsNET$ & $tsNET^*$ & \makecell{finetuned\\ $(DNN)^{2\textbf{*}}$} & \makecell{finetuned\\ $(DNN)^{2}$} \\
\midrule
$tsNET$                                      &         &     0.412 &                                          0.0 &                                0.0 \\
$tsNET^*$                                    &         &           &                                          0.0 &                                0.0 \\
\makecell{finetuned\\ $(DNN)^{2\textbf{*}}$} &         &           &                                              &                                0.0 \\
\makecell{finetuned\\ $(DNN)^{2}$}           &         &           &                                              &                                    \\
\bottomrule
\end{tabular}
}
\end{table}
\begin{table}[!h]
\centering
\caption{Conover-Iman post-hoc test p-values for Aspect ratio in Section 4.5. Significant threshold is $\alpha = 0.05$.}
\resizebox{\columnwidth}{!}{
\begin{tabular}{lllll}
\toprule
{} & $tsNET$ & $tsNET^*$ & \makecell{finetuned\\ $(DNN)^{2\textbf{*}}$} & \makecell{finetuned\\ $(DNN)^{2}$} \\
\midrule
$tsNET$                                      &         &     0.001 &                                          0.0 &                                0.0 \\
$tsNET^*$                                    &         &           &                                          0.0 &                                0.0 \\
\makecell{finetuned\\ $(DNN)^{2\textbf{*}}$} &         &           &                                              &                                0.0 \\
\makecell{finetuned\\ $(DNN)^{2}$}           &         &           &                                              &                                    \\
\bottomrule
\end{tabular}
}
\end{table}
\begin{table}[!h]
\centering
\caption{Conover-Iman post-hoc test p-values for Cross. number in Section 4.5. Significant threshold is $\alpha = 0.05$.}
\resizebox{\columnwidth}{!}{
\begin{tabular}{lllll}
\toprule
{} & $tsNET$ & $tsNET^*$ & \makecell{finetuned\\ $(DNN)^{2\textbf{*}}$} & \makecell{finetuned\\ $(DNN)^{2}$} \\
\midrule
$tsNET$                                      &         &     0.246 &                                        0.958 &                              0.001 \\
$tsNET^*$                                    &         &           &                                        0.268 &                              0.000 \\
\makecell{finetuned\\ $(DNN)^{2\textbf{*}}$} &         &           &                                              &                              0.000 \\
\makecell{finetuned\\ $(DNN)^{2}$}           &         &           &                                              &                                    \\
\bottomrule
\end{tabular}
}
\end{table}
\begin{table}[!h]
\centering
\caption{Conover-Iman post-hoc test p-values for Angular res. in Section 4.5. Significant threshold is $\alpha = 0.05$.}
\resizebox{\columnwidth}{!}{
\begin{tabular}{lllll}
\toprule
{} & $tsNET$ & $tsNET^*$ & \makecell{finetuned\\ $(DNN)^{2\textbf{*}}$} & \makecell{finetuned\\ $(DNN)^{2}$} \\
\midrule
$tsNET$                                      &         &      0.58 &                                        0.197 &                                0.0 \\
$tsNET^*$                                    &         &           &                                        0.462 &                                0.0 \\
\makecell{finetuned\\ $(DNN)^{2\textbf{*}}$} &         &           &                                              &                                0.0 \\
\makecell{finetuned\\ $(DNN)^{2}$}           &         &           &                                              &                                    \\
\bottomrule
\end{tabular}
}
\end{table}
\begin{table}[!h]
\centering
\caption{Conover-Iman post-hoc test p-values for Cluster overlap in Section 4.5. Significant threshold is $\alpha = 0.05$.}
\resizebox{\columnwidth}{!}{
\begin{tabular}{lllll}
\toprule
{} & $tsNET$ & $tsNET^*$ & \makecell{finetuned\\ $(DNN)^{2\textbf{*}}$} & \makecell{finetuned\\ $(DNN)^{2}$} \\
\midrule
$tsNET$                                      &         &     0.688 &                                        0.058 &                                0.0 \\
$tsNET^*$                                    &         &           &                                        0.022 &                                0.0 \\
\makecell{finetuned\\ $(DNN)^{2\textbf{*}}$} &         &           &                                              &                                0.0 \\
\makecell{finetuned\\ $(DNN)^{2}$}           &         &           &                                              &                                    \\
\bottomrule
\end{tabular}
}
\end{table}
\begin{table}[!h]
\centering
\caption{Conover-Iman post-hoc test p-values for Neighb. pres. in Section 4.5. Significant threshold is $\alpha = 0.05$.}
\resizebox{\columnwidth}{!}{
\begin{tabular}{lllll}
\toprule
{} & $tsNET$ & $tsNET^*$ & \makecell{finetuned\\ $(DNN)^{2\textbf{*}}$} & \makecell{finetuned\\ $(DNN)^{2}$} \\
\midrule
$tsNET$                                      &         &       0.0 &                                        0.515 &                                0.0 \\
$tsNET^*$                                    &         &           &                                        0.002 &                                0.0 \\
\makecell{finetuned\\ $(DNN)^{2\textbf{*}}$} &         &           &                                              &                                0.0 \\
\makecell{finetuned\\ $(DNN)^{2}$}           &         &           &                                              &                                    \\
\bottomrule
\end{tabular}
}
\end{table}
\begin{table}[!h]
\centering
\caption{Conover-Iman post-hoc test p-values for Execution time in Section 4.5. Significant threshold is $\alpha = 0.05$.}
\resizebox{\columnwidth}{!}{
\begin{tabular}{lllll}
\toprule
{} & $tsNET$ & $tsNET^*$ & \makecell{finetuned\\ $(DNN)^{2\textbf{*}}$} & \makecell{finetuned\\ $(DNN)^{2}$} \\
\midrule
$tsNET$                                      &         &       0.0 &                                          0.0 &                                0.0 \\
$tsNET^*$                                    &         &           &                                          0.0 &                                0.0 \\
\makecell{finetuned\\ $(DNN)^{2\textbf{*}}$} &         &           &                                              &                                0.0 \\
\makecell{finetuned\\ $(DNN)^{2}$}           &         &           &                                              &                                    \\
\bottomrule
\end{tabular}
}
\end{table}
\clearpage\subsection{Comparison with state-of-the-art methods}
\label{sec:bench3}
\begin{table}[!h]
\centering
\caption{Performances ($average \pm standard\:deviation$) of the different $(DNN)^2$ instances compared in Section 4.6.}
\resizebox{\columnwidth}{!}{
\begin{tabular}{llllllll}
\toprule
{} &                                 Stress &              \makecell{Aspect\\ ratio} &               \makecell{Cross.\\ number} &              \makecell{Angular\\ res.} &           \makecell{Cluster\\ overlap} &             \makecell{Neighb.\\ pres.} &               \makecell{Execution\\ time} \\
                                             &                                        &                                        &                                          &                                        &                                        &                                        &                                           \\
\midrule
$S\_GD^2$                                    &  \makecell{$0.066$ \\ $\pm$ \\$0.027$} &  \makecell{$0.263$ \\ $\pm$ \\$0.123$} &   \makecell{$32.15$ \\ $\pm$ \\$36.599$} &  \makecell{$0.812$ \\ $\pm$ \\$0.208$} &  \makecell{$0.583$ \\ $\pm$ \\$0.204$} &  \makecell{$0.439$ \\ $\pm$ \\$0.181$} &      \makecell{$1.133$ \\ $\pm$ \\$0.91$} \\
\midrule
GEM                                          &   \makecell{$0.24$ \\ $\pm$ \\$0.062$} &  \makecell{$0.573$ \\ $\pm$ \\$0.197$} &  \makecell{$54.407$ \\ $\pm$ \\$61.173$} &  \makecell{$0.972$ \\ $\pm$ \\$0.034$} &  \makecell{$0.722$ \\ $\pm$ \\$0.162$} &  \makecell{$0.617$ \\ $\pm$ \\$0.123$} &     \makecell{$5.223$ \\ $\pm$ \\$3.832$} \\
\midrule
PivotMDS                                     &  \makecell{$0.104$ \\ $\pm$ \\$0.035$} &  \makecell{$0.298$ \\ $\pm$ \\$0.125$} &   \makecell{$38.741$ \\ $\pm$ \\$43.56$} &  \makecell{$0.978$ \\ $\pm$ \\$0.088$} &  \makecell{$0.623$ \\ $\pm$ \\$0.202$} &    \makecell{$0.49$ \\ $\pm$ \\$0.17$} &     \makecell{$0.546$ \\ $\pm$ \\$0.478$} \\
\midrule
\makecell{finetuned\\ $(DNN)^{2\textbf{*}}$} &  \makecell{$0.115$ \\ $\pm$ \\$0.046$} &  \makecell{$0.229$ \\ $\pm$ \\$0.105$} &  \makecell{$30.625$ \\ $\pm$ \\$34.824$} &  \makecell{$0.917$ \\ $\pm$ \\$0.138$} &  \makecell{$0.541$ \\ $\pm$ \\$0.206$} &  \makecell{$0.409$ \\ $\pm$ \\$0.136$} &    \makecell{$25.145$ \\ $\pm$ \\$8.362$} \\
\midrule
\makecell{finetuned\\ $(DNN)^{2}$}           &   \makecell{$0.128$ \\ $\pm$ \\$0.06$} &  \makecell{$0.294$ \\ $\pm$ \\$0.134$} &  \makecell{$36.343$ \\ $\pm$ \\$39.879$} &  \makecell{$0.969$ \\ $\pm$ \\$0.092$} &   \makecell{$0.58$ \\ $\pm$ \\$0.197$} &  \makecell{$0.468$ \\ $\pm$ \\$0.154$} &    \makecell{$20.98$ \\ $\pm$ \\$10.326$} \\
\midrule
t-SNE                                        &   \makecell{$0.56$ \\ $\pm$ \\$0.771$} &  \makecell{$0.276$ \\ $\pm$ \\$0.158$} &  \makecell{$69.119$ \\ $\pm$ \\$48.878$} &   \makecell{$0.97$ \\ $\pm$ \\$0.038$} &  \makecell{$0.598$ \\ $\pm$ \\$0.252$} &  \makecell{$0.584$ \\ $\pm$ \\$0.097$} &  \makecell{$166.522$ \\ $\pm$ \\$71.723$} \\
\bottomrule
\end{tabular}
}
\end{table}
\begin{table}[!h]
\centering
\caption{Conover-Iman post-hoc test p-values for Stress in Section 4.6. Significant threshold is $\alpha = 0.05$.}
\resizebox{\columnwidth}{!}{
\begin{tabular}{lllllll}
\toprule
{} & $S\_GD^2$ & GEM & PivotMDS & \makecell{finetuned\\ $(DNN)^{2\textbf{*}}$} & \makecell{finetuned\\ $(DNN)^{2}$} & t-SNE \\
\midrule
$S\_GD^2$                                    &           & 0.0 &      0.0 &                                          0.0 &                                0.0 & 0.000 \\
GEM                                          &           &     &      0.0 &                                          0.0 &                                0.0 & 0.022 \\
PivotMDS                                     &           &     &          &                                          0.0 &                                0.0 & 0.000 \\
\makecell{finetuned\\ $(DNN)^{2\textbf{*}}$} &           &     &          &                                              &                                0.0 & 0.000 \\
\makecell{finetuned\\ $(DNN)^{2}$}           &           &     &          &                                              &                                    & 0.000 \\
t-SNE                                        &           &     &          &                                              &                                    &       \\
\bottomrule
\end{tabular}
}
\end{table}
\begin{table}[!h]
\centering
\caption{Conover-Iman post-hoc test p-values for Aspect ratio in Section 4.6. Significant threshold is $\alpha = 0.05$.}
\resizebox{\columnwidth}{!}{
\begin{tabular}{lllllll}
\toprule
{} & $S\_GD^2$ & GEM & PivotMDS & \makecell{finetuned\\ $(DNN)^{2\textbf{*}}$} & \makecell{finetuned\\ $(DNN)^{2}$} & t-SNE \\
\midrule
$S\_GD^2$                                    &           & 0.0 &      0.0 &                                          0.0 &                              0.000 & 0.001 \\
GEM                                          &           &     &      0.0 &                                          0.0 &                              0.000 & 0.000 \\
PivotMDS                                     &           &     &          &                                          0.0 &                              0.052 & 0.000 \\
\makecell{finetuned\\ $(DNN)^{2\textbf{*}}$} &           &     &          &                                              &                              0.000 & 0.000 \\
\makecell{finetuned\\ $(DNN)^{2}$}           &           &     &          &                                              &                                    & 0.000 \\
t-SNE                                        &           &     &          &                                              &                                    &       \\
\bottomrule
\end{tabular}
}
\end{table}
\begin{table}[!h]
\centering
\caption{Conover-Iman post-hoc test p-values for Cross. number in Section 4.6. Significant threshold is $\alpha = 0.05$.}
\resizebox{\columnwidth}{!}{
\begin{tabular}{lllllll}
\toprule
{} & $S\_GD^2$ & GEM & PivotMDS & \makecell{finetuned\\ $(DNN)^{2\textbf{*}}$} & \makecell{finetuned\\ $(DNN)^{2}$} & t-SNE \\
\midrule
$S\_GD^2$                                    &           & 0.0 &      0.0 &                                        0.362 &                               0.00 &   0.0 \\
GEM                                          &           &     &      0.0 &                                        0.000 &                               0.00 &   0.0 \\
PivotMDS                                     &           &     &          &                                        0.000 &                               0.57 &   0.0 \\
\makecell{finetuned\\ $(DNN)^{2\textbf{*}}$} &           &     &          &                                              &                               0.00 &   0.0 \\
\makecell{finetuned\\ $(DNN)^{2}$}           &           &     &          &                                              &                                    &   0.0 \\
t-SNE                                        &           &     &          &                                              &                                    &       \\
\bottomrule
\end{tabular}
}
\end{table}
\begin{table}[!h]
\centering
\caption{Conover-Iman post-hoc test p-values for Angular res. in Section 4.6. Significant threshold is $\alpha = 0.05$.}
\resizebox{\columnwidth}{!}{
\begin{tabular}{lllllll}
\toprule
{} & $S\_GD^2$ & GEM & PivotMDS & \makecell{finetuned\\ $(DNN)^{2\textbf{*}}$} & \makecell{finetuned\\ $(DNN)^{2}$} & t-SNE \\
\midrule
$S\_GD^2$                                    &           & 0.0 &      0.0 &                                          0.0 &                                0.0 & 0.000 \\
GEM                                          &           &     &      0.0 &                                          0.0 &                                0.0 & 0.006 \\
PivotMDS                                     &           &     &          &                                          0.0 &                                0.0 & 0.000 \\
\makecell{finetuned\\ $(DNN)^{2\textbf{*}}$} &           &     &          &                                              &                                0.0 & 0.000 \\
\makecell{finetuned\\ $(DNN)^{2}$}           &           &     &          &                                              &                                    & 0.000 \\
t-SNE                                        &           &     &          &                                              &                                    &       \\
\bottomrule
\end{tabular}
}
\end{table}
\begin{table}[!h]
\centering
\caption{Conover-Iman post-hoc test p-values for Cluster overlap in Section 4.6. Significant threshold is $\alpha = 0.05$.}
\resizebox{\columnwidth}{!}{
\begin{tabular}{lllllll}
\toprule
{} & $S\_GD^2$ & GEM & PivotMDS & \makecell{finetuned\\ $(DNN)^{2\textbf{*}}$} & \makecell{finetuned\\ $(DNN)^{2}$} & t-SNE \\
\midrule
$S\_GD^2$                                    &           & 0.0 &      0.0 &                                          0.0 &                              0.178 & 0.000 \\
GEM                                          &           &     &      0.0 &                                          0.0 &                              0.000 & 0.000 \\
PivotMDS                                     &           &     &          &                                          0.0 &                              0.000 & 0.133 \\
\makecell{finetuned\\ $(DNN)^{2\textbf{*}}$} &           &     &          &                                              &                              0.000 & 0.000 \\
\makecell{finetuned\\ $(DNN)^{2}$}           &           &     &          &                                              &                                    & 0.000 \\
t-SNE                                        &           &     &          &                                              &                                    &       \\
\bottomrule
\end{tabular}
}
\end{table}
\begin{table}[!h]
\centering
\caption{Conover-Iman post-hoc test p-values for Neighb. pres. in Section 4.6. Significant threshold is $\alpha = 0.05$.}
\resizebox{\columnwidth}{!}{
\begin{tabular}{lllllll}
\toprule
{} & $S\_GD^2$ & GEM & PivotMDS & \makecell{finetuned\\ $(DNN)^{2\textbf{*}}$} & \makecell{finetuned\\ $(DNN)^{2}$} & t-SNE \\
\midrule
$S\_GD^2$                                    &           & 0.0 &      0.0 &                                          0.0 &                                0.0 &   0.0 \\
GEM                                          &           &     &      0.0 &                                          0.0 &                                0.0 &   0.0 \\
PivotMDS                                     &           &     &          &                                          0.0 &                                0.0 &   0.0 \\
\makecell{finetuned\\ $(DNN)^{2\textbf{*}}$} &           &     &          &                                              &                                0.0 &   0.0 \\
\makecell{finetuned\\ $(DNN)^{2}$}           &           &     &          &                                              &                                    &   0.0 \\
t-SNE                                        &           &     &          &                                              &                                    &       \\
\bottomrule
\end{tabular}
}
\end{table}
\begin{table}[!h]
\centering
\caption{Conover-Iman post-hoc test p-values for Execution time in Section 4.6. Significant threshold is $\alpha = 0.05$.}
\resizebox{\columnwidth}{!}{
\begin{tabular}{lllllll}
\toprule
{} & $S\_GD^2$ & GEM & PivotMDS & \makecell{finetuned\\ $(DNN)^{2\textbf{*}}$} & \makecell{finetuned\\ $(DNN)^{2}$} & t-SNE \\
\midrule
$S\_GD^2$                                    &           & 0.0 &      0.0 &                                          0.0 &                                0.0 &   0.0 \\
GEM                                          &           &     &      0.0 &                                          0.0 &                                0.0 &   0.0 \\
PivotMDS                                     &           &     &          &                                          0.0 &                                0.0 &   0.0 \\
\makecell{finetuned\\ $(DNN)^{2\textbf{*}}$} &           &     &          &                                              &                                0.0 &   0.0 \\
\makecell{finetuned\\ $(DNN)^{2}$}           &           &     &          &                                              &                                    &   0.0 \\
t-SNE                                        &           &     &          &                                              &                                    &       \\
\bottomrule
\end{tabular}
}
\end{table}
